# Supplementary material for: Cerberus: Query-driven Scalable Vulnerability Detection in OAuth Service Provider Implementations
Source: arXiv:2110.01005 source file (2023-08-29)
Supplement: Supplementary file 1 [file appendix.tex]

\clearpage
% \appendix
 \begin{appendices}

\section{Appendix: Security Properties for \oauthserver}~\label{apx:properties}
In this section, we describe more details about the properties in Table~\ref{tab:list-of-properties}. We identify these properties by analyzing standard OAuth specification~\cite{rfc6749, rfc6819} and Security best practices~\cite{oauth-best-practice}.

\paragraph{Property P1:} \emph{Redirect URI must match client's registered uri.}
With the redirect URI parameter provided by the client at the authorization request endpoint, the \oauthserver must check if the URI is the same as the one registered to the client. 
As mentioned by the specification~\cite{rfc6749}, the \oauthserver must compare and match the redirect URI against the registered redirection URI. Failure to validate the redirect URI properly involves severe security implications. We demonstrate an attack example caused by incorrect redirect URI validation in Appendix~\ref{apx:attacks}. Additionally, OAuth security best practices~\cite{oauth-best-practice} states the complexity of implementing and managing to match URI correctly obviously causes security issues. The server must compare the two URIs using simple string comparison as defined in RFC-3986. However, if the redirect URI validation fails, the \oauthserver should inform the resource owner and avoid making an automatic redirection to the redirect URI, as the URI is invalid and potentially be manipulated by the attackers. According to the specification~\cite{rfc6749}, ``if the request fails due to a missing, invalid, or mismatching redirection URI, ... the server should inform the resource owner of the error and must not automatically redirect the user-agent to the invalid redirection URI.''
\paragraph{Property P2:} \emph{Redirect URI must be an absolute URI.}
OAuth specification~\cite{rfc6749} requires that, ``the redirection endpoint URI must be an absolute URI as defined by RFC-3986 Section 4.3.'' The URI value should not include a fragment component, since allowing the fragment in the redirect URI enables the attacker to utilize the open redirector of the user agent and intercept the authorization code or token attached with the redirect URI. These validation checks for redirect URI add an extra layer of security against the redirect URI manipulation by the attacker during the authorization request. An attack example for violating the redirect URI properties is demonstrated in Appendix~\ref{apx:attacks}.
\paragraph{Property P3:} \emph{Authorization code must be single-use.}
The specification states, ``the client must not use authorization code more than once. If an authorization code is used more than once, the server must deny the request.''. In addition to this check, the specification also recommends that if the server observes multiple attempts to exchange an authorization code for an access token, the server should reject the request with an error message and should revoke all access tokens already granted based on the compromised authorization code.'' This allows the server to protect the resources of a potentially compromised resource owner. Typically, the server stores the authorization code and the associated authorization information in its storage (e.g., database) during the authorization request and removes the code from the storage once it is used at the token endpoint by the client. Thus, if the submitted code at the token endpoint does not return any associated information from the storage, the server determines a potential malicious attempt of the authorization code being used for multiple times.

\paragraph{Property P4:} \emph{Authorization code must be bound to client.}
As the specification states, ``authorization code is bound to the client identifier''. Precisely, authorization code submitted at token endpoint should be issued to the same client during the authorization request. As discussed in the authorization code injection attack scenario in Appendix~\ref{apx:attacks}, this check by the \oauthserver prevents the attacker from injecting an authorization code that was obtained from a different client application under the control of the attacker. To satisfy this property, the server must check that the client that initiated the token request with an authorization code is identical to the client to which the code was issued to.

% {\footnotesize
% \begin{verbatim}
% 1. P4 :- invoke(L1, token_req), OAuthTag(L2, code),  
% 2.       OAuthTag(L3,client_code), invoke(L4,gen_token),
% 3.       error(L5, _), branch(L6,X,L4,L5), followBy(L1,L2)
% 4.       followBy(L1,L3), depOn(L2,X), depOn(L3,X).
% \end{verbatim}
% }

% (\tamjid{explaining the query in natural language so that expressing them in formal language becomes easier})\\
% We basically need to check the following in this query:\\
% 1. A getField statement for \textit{request.code} flows to a function for database read operation (fetch code\_info for the request.code from the database).\\
% 2. A getField statement to access code\_info.client flows to a conditional statement with inequality check.\\
% 3. A getField statement to access \textit{request.client} flows to the same conditional statement with inequality check.\\
% 4. If the condition is taken (\textit{request.client} not equals to code\_info.client), then Error() function is invoked to deny the request.\\

% A code example for this check is shown in Figure~\ref{fig:code-example-token-req}[Line 14].
% Query:\\
% $get\_field(request, code) \rightarrow invoke\_stmt(read()) \wedge$\\
% $v = invoke\_stmt(read()) \rightarrow get\_field(v, client) \wedge$\\
% $get\_field(v, client) \rightarrow cond\_stmt(P) \wedge$\\
% $get\_field(request, client) \rightarrow cond\_stmt(P) \wedge$\\
% $\ IF (P), THEN \{invoke\_stmt(Error)\}$\\
% Here, predicate P in the conditional statement checks inequality.

\paragraph{Property (P5):} \emph{Authorization code must be bound to the redirect URI.}
OAuth specification requires the \oauthserver to ensure that the authorization code presented at the token endpoint is associated with the redirect URI submitted during the authorization request. Particularly, this validation ensures the authorization code used by the client was initially issued to the redirect URI that belongs to the client. This check is important to prevent the attacker from injecting an authorization code obtained by manipulating the redirect URI during the authorization request. As discussed in the authorization code injection attack scenario in Appendix~\ref{apx:attacks}, the legitimate client would send the same redirect URI is used for the authorization request, but it would not match the manipulated redirect URI used by the attacker to obtain the code. Therefore, the checking at the token endpoint of the \oauthserver would fail, and the token request would be rejected. 
% (\tamjid{explaining the query in natural language so that expressing them in formal language becomes easier})\\
% This query is similar to the previous one, except we check redirect URI instead of client information.

% {\footnotesize
% \begin{verbatim}
% 1. P5 :- invoke(L1, token_req), OAuthTag(L2, code),  
% 2.       OAuthTag(L3,client_URI), invoke(L4,gen_token),
% 3.       error(L5, _), branch(L6,X,L4,L5), followBy(L1,L2)
% 4.       followBy(L1,L3), depOn(L2,X), depOn(L3,X).
% \end{verbatim}
% }

% An attack example (authorization code injection) for violating the above-mentioned properties of authorization code is demonstrated in Appendix~\ref{apx:attacks}.\\

\paragraph{PKCE.} Satisfying the above properties is not enough to prevent the authorization code injection attack (Appendix~\ref{apx:attacks}) for public clients (e.g., native desktop apps) as they may not have a server-side counterpart and cannot securely store the client credentials. Such clients often store the credentials as a hard-coded variable in the source code, which allows the attacker extracts the credentials and effectively break the client authentication during the token request. PKCE allows the \oauthserver to authenticate the client at the token request without the client credentials and prevents attackers from performing authorization code injection attacks. OAuth security current best practices~\cite{oauth-best-practice} states that ``authorization servers must support PKCE''. Although it was originally designed solely for native applications, it is now recommended to use PKCE for regular authorization code grant type. PKCE involves implementation at authorization and token endpoint and we describe the PKCE properties for both endpoints as following:

\paragraph{Property P6:} \emph{Validate and store PKCE parameters at the authorization endpoint.}
% Public clients (e.g., mobile apps, native desktop apps etc.) cannot maintain client-side confidentiality during OAuth authorization flow. Consequently, public clients using the Authorization Code Grant are vulnerable to severe OAuth attacks such as authorization code interception attack~\cite{rfc7636}. These attacks lead attackers to steal the access token and have been observed in the wild. 
% To mitigate the code injection attacks, OAuth specification~\cite{rfc7636} recommends OAuth servers to use Proof Key for Code Exchange (PKCE) extension for Authorization Code Grant flow. 
PKCE utilizes a dynamically created cryptographic random key called $code\_verifier$.  For every authorization request, a unique $code\_verifier$ is created by, and its transformed value, called $code\_challenge$ is sent to the server to obtain the authorization code. Clients often include the transformation method, called $code\_challenge\_method$ with the authorization request. These parameters must be stored so that they can be accessed to verify the subsequent request received at the token endpoint. 

% {\footnotesize
% \begin{verbatim}
% 1. P6 :- invoke(L1, auth_req), OAuthTag(L2, code_chal),  
% 2.       OAuthTag(L3,code_chal_meth), sstore(L4,db),
% 3.       followBy(L1,L2), followBy(L1,L3),
% 4.       depOn(L2,L4), depOn(L3,L4).
% \end{verbatim}
% }

% (\tamjid{explaining the query in natural language so that expressing them in formal language becomes easier})\\
% To implement this property, the authorization server needs to associate the value of code challenge and code challenge method with the authorization code when it stores them in the database at the authorization endpoint, so that when clients submit the code at the token endpoint, authorization server can retrieve the corresponding code challenge to verify.\\
% 1. Return value of a function call that generates the code value flows to a database insert function.\\
% 2. getField statement for the $request.code\_challenge$ and getField statement for $request.code\_challenge\_method$ flows to the same database insert function.\\
% $[v = invoke\_stmt(generateCode)\wedge get\_field(request, code\_challenge) \wedge get\_field(request, code\_challenge\_method)] \rightarrow invoke\_stmt(read())$\\

\paragraph{Property P7:} \emph{Verify PKCE parameters at the token endpoint.}
At the token endpoint, along with the authorization code, the \oauthserver also receive a $code\_verifier$--the secret generated by the client before initiating the authorization request. The server transforms the $code\_verifier$ and compares it with the $code\_challenge$ which it received from the client in previous request (i.e., authorization). However, the server denies the request (with an error response) if the values do not match, as it implies the $code$ was not issued to the same client that made the request for the token. This approach eliminates the need to send the client secret at the token request endpoint to authenticate the client. The requirement to send client secret makes it difficult to store the secret securely, especially for public clients (e.g., mobile or native desktop apps) who cannot maintain client-side confidentiality. According to PKCE specification~\cite{rfc7636}, the value of $code\_challenge\_method$ that is used to transform the $code\_verifier$, can either be `S256' or `plain'. The `S256' is secure and recommended method since it protects against eavesdropping or intercepting the $code\_challenge$ and the challenge cannot be used without the $code\_verifier$. On the other hand, as the term suggests, `plain' does not provide any transformation of the $code\_verifier$, and therefore, the value of $code\_challenge$ is exactly the same as the value of $code\_verifier$. According to the PKCE specification for OAuth, ``\textit{plain} should not be used and exists only for compatibility with deployed implementations where the request path is already protected.'' Therefore, for this property, we only consider `S256' as the value of the $code\_challenge\_method$.

% The above property can be formally expressed using the following query:
%   \begin{align*}
%   & 1. \ \ \mathsf{Var} \ x, y, z, z_1, z_2, \mathsf{Stmt} \ s, \mathsf{Request} \ r\\
%   & 2. \ \ \assumesStmt{\mathsf{codeChallenge(x)} \land \mathsf{ifStmt(\_,z)} \land \mathsf{codeVerifier(y)}} \\
%   & 3. \ \ \assumesStmt{\mathsf{sha256(\_, z_1)} \land \mathsf{base64Encode(\_,z_2)}} \land \mathsf{isError}(s)\\
%     & 4. \ \ \letStmt{\mathsf{m}}{\mathsf{challengeMethod}(r)} \\
%   & 5. \ \ \ensuresStmt{ (m = ``SHA256") \rightarrow \mathsf{flowTo}(x,z) \land \mathsf{flowTo}(y,z_1)}  \\ 
%   & \land \mathsf{flowTo}(z_1, z_2) \land \mathsf{flowTo}(z_2, z) \land \mathsf{controlDep}(z,s) 
% \end{align*}

\paragraph{Property P8:} \emph{Use `$state$' parameter to provide CSRF protection.}
CSRF allows an attacker to cause the user agent of a victim user to follow a malicious URI (e.g., redirection) to a legitimate server. In the OAuth context, a CSRF attack allows the attacker to inject a request to the legitimate client's redirection URI with its own authorization code or access token. It causes the client to use an access token associated with the attacker's resources instead of the victim's resources. As mentioned in the OAuth specification, ``a CSRF attack against the server's authorization endpoint can result in an attacker obtaining end-user authorization for a malicious client without involving or alerting the end-user. The server must implement CSRF protection for its authorization endpoint. ''OAuth servers often do not require clients to provide `$state$' parameter during the authorization request. This string value parameter helps to maintain the state between the client's authorization request and the server's authorization response. Thus, it provides clients a protection mechanism from Cross-site request forgery (CSRF) attack~\cite{rfc6819}. The satisfy this property, the server checks if the `$state$' parameter is present at the authorization endpoint and it associates the parameter value with the response, so that the client can validate the authenticity of the response received from the server.

% {\footnotesize
% \begin{verbatim}
% 1. P8 :- invoke(L1, auth_req), OAuthTag(L2, state),  
% 2.       invoke(L3, redirect), error(L4,_), branch(L5,X,L3,L4),
% 3.       followBy(L1,L2), depOn(L2,X), depOn(L2,L3).
% \end{verbatim}
% }

\paragraph{Property P9:} \emph{Access tokens should be constrained to a certain client.}
A client-constrained access token limits the applicability of an access token to a particular client. In other words, instead of a portable and plain access token, the \oauthserver encrypts the token with a commonly distributed key between the client and the \oauthserver. This binding mechanism also allows the client to demonstrate the proof of possession when exchanging the access token for resources. There have been several proposed approaches to demonstrate the proof of possession for access token such as mutual-TLS~\cite{rfc8705} and signed HTTP requests~\cite{signed-http}. However, since the mutual TLS (also known as mTLS) is the most widely used and the only standardized client-constrained mechanism, in this paper, we consider the mutual TLS approach for implementing client-constrained approach, which is also recommended by the OAuth security current best practices~\cite{oauth-best-practice}. In the mutual TLS approach, the \oauthserver obtains the client's public key from the TLS stack during the token request at the token endpoint and associates the key with the access token before issuing the token to the client. This mechanism allows the server to verify the proof of possession when the token is submitted for requesting the resources. Therefore, an attacker can not inject a stolen access token to the legitimate client as the attack will be detected when the token is exchanged for the resources.
% To implement this property, the \oauthserver first obtains the client's certificate from the TLS stack during the token request. The server then decodes the certificate, hashes it and finally associate the hashed certificate with the access token.\\

% An example for implementing this property can be expressed as following:\\
% accessToken= generateToken(...);\\
% cert = request.getHeader("X-ClientCert");\\
% decodedCert = Base64.decode(cert);\\
% hashedCert = base64urlencode(sha256(decodedCert));\\
% accessToken.setCertificate(hashedCert);\\
% Using the query language and predicates defined in Section~\ref{sec:system}, the mutual TLS approach for the above property can be formally expressed using the following query:\\

% {\footnotesize
% \begin{verbatim}
% 1. P9 :- OAuthTag(L1, access_token),  
% 2.       OAuthTag(L2, client_cert), OAuthTag(L3, 
% 3.       b64_decode), OAuthTag(L4, b64_encode), 
% 4.       OAuthTag(L5, sha256),OAuthTag(L6, add_cert),
% 5.       FlowTo(L2,L3),FlowTo(L3,L5),FlowTo(L5,L4),
% 6.       FlowTo(L1,L6),FlowTo(L4,L6),
% \end{verbatim}
% }

% {\small
%   \begin{align*}
%   & 1. \ \ \mathsf{Var} \ x, y, z_1, z_2,z_3,z_4,z_5 , \mathsf{Request} \ r\\
%   & 2. \ \ \assumesStmt{\mathsf{isToken(x)} \land \mathsf{isCertificate(y)}} \\
%   & 3. \ \ \assumesStmt{\mathsf{base64Decode(\_, z_1)} \land  \mathsf{sha256(\_,z_2)}} \land\\
%   & \ \ \mathsf{base64Encode(\_,z_3)} \land \mathsf{addCertificate(\_,z_4,z_5)}\\
%   & 4. \ \ \ensuresStmt{ (\mathsf{clientCert(r,'ClientCert')}) \rightarrow \mathsf{dataDep(y,z_1)}} \land \\
%   & \ \ \mathsf{dataDep(z_1,z_2)} \land \mathsf{dataDep(z_2,z_3)} \land \mathsf{dataDep(x,z_4)} \land \\
%   & \ \ \mathsf{dataDep(z_3,z_5)}\\ 
% \end{align*}
% }

\paragraph{Property P10:} \emph{Access tokens should not be stored as clear-text.}
The \oauthserver must prevent the leakage of access tokens from its database. If the attacker gets access to the server's database, it can expose the access tokens of all the resource owners hosted by the corresponding server. The attacker might also steal the access token of a victim resource owner by performing an SQL injection attack. If the \oauthserver stores the access token in clear text, the attacker can use the token for performing an access token injection attack as described above. The standard security considerations for OAuth~\cite{rfc6819} recommends to ``store access token hashes only.'' However, prevention the common attacks such as SQL injection is out of the scope of this paper. Therefore, we focus on the mitigation of the OAuth attacks, such as access token injection. 
% {\footnotesize
% \begin{verbatim}
% 1. P10 :- OAuthTag(L1, access_token), invoke(L2, sha256),
% 2.        sstore(L3,db), depOn(L1,L2), depOn(L2,L3).
% \end{verbatim}
% }

% An example for implementing this property can be expressed as following:\\
% accessToken= generateToken(...);\\
% hashedToken = base64urlencode(sha256(accessToken));\\
% storeToken(hashedToken);\\

\section{Appendix: Attacks on \oauthserver}~\label{apx:attacks}
This section describes the common attacks for the \oauthserver. We describe an attack scenario and security impacts for each attack on different endpoints of the server.

% \subsubsection{Authorization Request endpoint.}
% Client uses the authorization request endpoint of OAuth server to obtain user authorization. This endpoint typically receives client\_id, redirect\_uri, response\_type and scope as request parameter, and upon authenticating users, it responds with authorization code or access token depending on the grant type. Since request to this endpoint results in transmission of sensitive OAuth-credentials, server must implement the sufficient validation of the received parameters to avoid severe security attacks such as access token hijacking. We describe the security relevant properties of the authorization request endpoint of the OAuth server as following:

\subsection{Redirect URI Manipulation:}
Lack of redirect URI validation (P1 \& P2) by the \oauthserver effectively breaks the client identification (authorization code grant) or authentication (implicit grant) and allows attackers to steal the authorization code or access token. Missing or incorrect validation of redirect URI allows the attacker to obtain the OAuth credentials by either (1) directly redirecting the user agent to a URI under the attacker's control or (2) exposing the credentials to an attacker by utilizing an open redirector at the client application by leveraging the way user agents handle URI fragments. For example, instead of complete redirect URIs, some servers allow clients to register to redirect URI patterns to support dynamic redirect URI for different sub-domains. Therefore, for the request at the authorization endpoint, the  server matches the redirect URI parameter value against the registered patterns. Although this approach allows the clients to register one pattern for all sub-domains or encode transaction state into redirect URI parameter, it opens a gateway for the attacker to obtain the authorization code or access token sent from the authorization endpoint. For example, for a client using authorization code grant type, an attack may work as following:

\subsubsection{Attack example.} Assume an honest client intends to use any sub-domain of \textit{honestclient.com} as redirect URI for their application and registers the redirect URI pattern \textit{https://*.honestclient.com/*} with the \oauthserver. The server, however, might interpret the wildcard syntax \textit{'*'} as a match for any character, and thereby, might recognize \textit{https://attacker.com/.honestclient.com/} as a valid redirect URI, even though \textit{attacker.com} is a different domain that the attacker could control. The attack scenario is illustrated in Fig.~\ref{fig:attack-redirect-uri}. First, the attacker takes a phishing approach (step A) to trick the resource owner to land on a malicious page that initiates an authorization request with the value of the $redirect\_uri$ parameter as \textit{https://attacker.com/.honestclient.com/}. The resource owner thinks of the phishing web page as from the legitimate client and authorizes the page (step B). The server compares the received redirect URI with the redirect URI pattern registered by the client and processes the authorization request. The resource owner may not notice the malicious redirect URI as for some user agents (e.g., Android WebView), the URI is not visible to the users. Therefore, the authorization code is issued (step C) by the server and directly sent to the attacker's domain. Now the attacker has the authorization code, which it may use to impersonate the client and exchange the authorization code for the access token at the token endpoint of the same server. If the client uses the implicit grant type, this attack can even be worse as the attacker can directly obtain the access token using this approach. 
\begin{figure}[!t]
  \includegraphics[width=\linewidth]{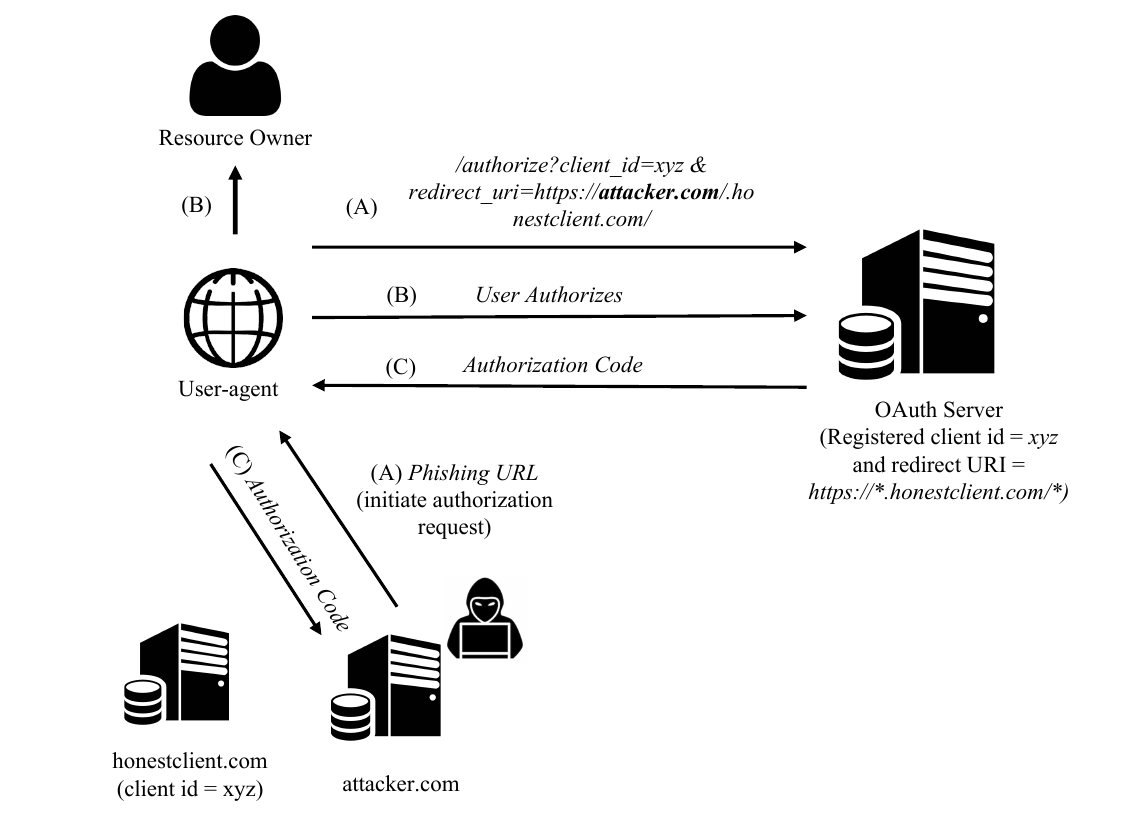}
  \caption{An attack scenario where attacker initiates an authorization request with a manipulated redirect URI parameter and obtains the authorization code of a victim resource owner.}
  \label{fig:attack-redirect-uri}
\end{figure}

\subsection{Authorization Code Injection:}
Violation of authorization code properties (P3, P4\& P5) can result in an authorization code injection attack. In this attack, the attacker attempts to inject a stolen authorization code it obtained from the authorization endpoint of the server. There can be two attack scenarios for authorization code injection. First, an \oauthserver with minimal security may not associate an authorization code with a particular client. Therefore, the attacker can easily obtain the access token from the token endpoint as it does not require authentication for any client. In the second scenario, the server binds the code with a particular client so that the code cannot be exchanged for an access token without an authenticated client. Therefore, in this attack scenario, the goal is to associate the attacker's session at the client with the victim resource owner, as the attacker cannot exchange the code for an access token by himself. This kind of attack is also useful when the attacker wants to impersonate his victim of a certain client application or a website. An authorization code injection attack may work as follows:

\subsubsection{Attack example.} To conduct an authorization code injection, the attacker first obtains an authorization code by performing a code intercept attack by manipulating the redirect URI as discussed above. Then he performs a regular authorization process with a legitimate client on his device. Since the authorization response passes through the attacker's device, the attacker can use any tool to intercept and manipulate the response to this end. The attacker injects the stolen authorization code in the response of the server to the legitimate client. The legitimate client then sends the code with the client's credentials to the token endpoint of the \oauthserver. The server checks the authenticity of the client's credentials and if the code is issued to the particular client. If all checks succeed, server issues the access token to the client. Thus, the attacker has now successfully associated his session with the legitimate client with the victim resource owner.

\subsection{Access Token Injection:}
Violation of token properties (P9 \& P10) can result in access token injection attack. The server needs to implement measures to protect its clients from this attack. In access token injection attack, the attacker attempts to impersonate a resource owner by injecting a stolen access token into a legitimate client. An attack scenario of access token injection is discussed as follows:

\subsubsection{Attack example.} To conduct an access token injection attack, the attacker first initiates the OAuth flow from a client application that uses the implicit grant for the authorization request. After successful authorization is obtained from the resource owner, the server issues an access token to the client application by using URI redirection through the user agent. The attacker modifies the response from the server and replaces the access token value with a stolen or leaked access token. As the attacker keeps all other parameters (e.g., \textit{state} parameter) the same as the original request, the client does not recognize the response as a CSRF attack and uses the access token injected by the attacker. 

Although clients using the implicit grant are most vulnerable to the access token injection attack, such attacks are also common for the clients that use the authorization code grant in an incorrect way. A significant number of mobile applications have been observed~\cite{chen2014oauth, DBLP:conf/kbse/RahatFT19} to use an incorrect authorization code grant where authorization request and token request are both made from the client applications. Since the attacker can modify any request or response at the client application, they can conduct the access token injection attack when the client uses an implicit grant or an incorrect authorization code grant. The authorization should implement the following properties to mitigate the risk of access token injection attacks.

\end{appendices}
